# Supplementary material for: Integrated waveguides and deterministically positioned nitrogen vacancy centers in diamond created by femtosecond laser writing
Source: arXiv:1701.05885 ancillary file (2018-03-12)
Supplement: Supplementary file 1 [file wgnv-supplemental.pdf]

**Supplementary Material:**

**Integrated waveguides and deterministically positioned nitrogen vacancy centers in diamond created by femtosecond laser writing**

J. P. HADDEN,<sup>1, a)</sup> V. BHARADWAJ,<sup>2, a)</sup> B. SOTILLO,<sup>2</sup> S. RAMPINI,<sup>2</sup> R. OSELLAME,<sup>2</sup> J. WITMER,<sup>1, b)</sup> H. JAYAKUMAR,<sup>1, c)</sup> T. T. FERNANDEZ,<sup>2</sup> A. CHIAPPINI,<sup>3</sup> C. ARMELLINI,<sup>3</sup> M. FERRARI,<sup>3</sup> R. RAMPONI,<sup>2</sup> P. E. BARCLAY,<sup>1</sup> and S. M. EATON<sup>2</sup>

(Corresponding author: [jpe.hadden@gmail.com](mailto:jpe.hadden@gmail.com))

<sup>1)</sup>*Institute for Quantum Science and Technology, University of Calgary, Calgary, T2N 1N4, Canada.*

<sup>2)</sup>*Istituto di Fotonica e Nanotecnologie-Consiglio Nazionale delle Ricerche (IFN-CNR) and Dipartimento di Fisica - Politecnico di Milano, Piazza Leonardo da Vinci 32, Milano, 20133, Italy*

<sup>3)</sup>*Istituto di Fotonica e Nanotecnologie (IFN-CNR), CSMFO and FBK-CMM, Via alla Cascata, 56/C, Trento, 38123, Italy*

(Dated: 7 March 2018)

---

<sup>a)</sup>These authors contributed equally to this publication

<sup>b)</sup>Currently at Ginzton Laboratory, Stanford University, Stanford, CA 94305, USA

<sup>c)</sup>Currently at Department of Physics, City University of New York (CUNY)-City College of New York, New York, NY 10031, USA

## I. DEVICE FABRICATION

The femtosecond laser used for waveguide writing was a regeneratively amplified Yb:KGW system (Pharos, Light Conversion) with 230 fs pulse duration, 515 nm wavelength and 500 kHz repetition rate. The femtosecond laser pulses were focused below the diamond surface with a 1.25 NA oil immersion lens (RMS100X-O 100 $\times$  Plan Achromat Oil Immersion Objective, Olympus). Computer-controlled 3-axis motion stages (ABL1000, Aerotech) were used to translate the quantum grade diamond sample (2 mm  $\times$  2 mm  $\times$  0.3 mm, nitrogen impurities <5 ppb, MB optics) transversely relative to the laser to form the optical waveguides.

The optical waveguide was formed at 25  $\mu\text{m}$  depth with processing conditions of 500 kHz repetition rate, 60 nJ pulse energy, and 0.5 mm s $^{-1}$  scan speed, corresponding to approximately 1000 pulses within the scanned focal spot. Because focused femtosecond laser pulses yield an amorphization/graphitization in crystalline diamond, the type II geometry<sup>1</sup> was adopted, where two closely spaced laser-written modification lines provide optical confinement. To achieve single mode guiding of visible light, 13  $\mu\text{m}$  separation between the laser-formed modification lines was used. A lower pulse energy was required than in our previous study<sup>2</sup> because of the shallower depth, resulting in reduced spherical aberration and therefore less distortion in the intensity distribution at the focus.

The near-field intensity profile of the single transverse waveguide mode was measured by imaging the output facet with a 0.65 NA 60 $\times$  asphere to a CCD (SP620U, Spiricon). The mode field diameter (MFD) for the nearly circular mode was 9.5  $\mu\text{m}$  at 635 nm wavelength. MFD measurements were made using the  $D4\sigma$  (second moment width) calculation from the beam profiling software (BeamGage, Spiricon), approximately equal to the  $1/e^2$  diameter for the nearly Gaussian mode. The insertion loss was 5.4 dB at 635 nm wavelength (TLS001-635, Thorlabs) for the TM polarization launched with a PM fiber. Accounting for the 2.0 dB coupling loss per facet due to mode mismatch between the fiber (MFD 4.6  $\mu\text{m}$ ) and optical waveguide mode (MFD 9.5  $\mu\text{m}$ ), and the Fresnel loss (0.3 dB/facet) due to the refractive index difference between the optical fiber/index matching oil ( $n = 1.5$ ) and diamond ( $n = 2.4$ ), we infer a propagation loss of 4.2 dB/cm.

Using the same femtosecond laser setup, single-pulse exposures were inscribed within the optical waveguide to induce vacancies in the diamond lattice. The pulse energy used was

28 nJ. Five identical static exposures separated by 20  $\mu\text{m}$  were written in order to study reproducibility in forming single NV centers within the waveguiding region. The depth of the static exposures was 25  $\mu\text{m}$ , centered within the cross section of the laser-written waveguide. Markers visible in our imaging system were inscribed (100 nJ pulse energy, 25 pulses) outside of the waveguide to locate the single pulse exposures, which are not visible to wide-field illuminated optical microscopy.

The diamond sample was subsequently annealed in order to form NV centers. Vacancies, which become mobile above 600  $^{\circ}\text{C}$ , are captured by substitutional nitrogen<sup>3</sup>. In a sample of this type there can be 100-1000 nitrogen impurities present within the ( $\sim 1 \mu\text{m}^3$ ) focal volume of the focused femtosecond laser beam. It has been shown that annealing at higher temperatures (1000  $^{\circ}\text{C}$  and above) can improve the optical linewidths and spin coherence times of the NV centers, as other vacancy complexes which can be detrimental are annealed out<sup>4,5</sup>. The annealing was performed in a tubular horizontal furnace (LTF15/50/450, Lenton) at 1000  $^{\circ}\text{C}$  for three hours in a nitrogen atmosphere, to avoid oxidation of the diamond surface. Further details on the annealing process can be found in our previous work<sup>6</sup>.

At such temperatures, the bulk material does not suffer structural changes or graphitization<sup>7</sup>. Previous studies in other crystals have shown that high temperature annealing can erase waveguides produced by femtosecond laser irradiation<sup>8,9</sup>, due to the recovery of the crystalline structure. In the case of diamond, the laser modification lines remain after annealing, as the lattice is not restored<sup>10</sup>. From  $\mu\text{Raman}$  measurements performed on the laser-induced modification lines, we observed the formation of a higher concentration of graphite nanoclusters after annealing, consistent with other studies<sup>10,11</sup>.

Even with the increased graphite inside the modification lines,  $\mu\text{Raman}$  shows similar diamond Raman peak width (i.e. crystal quality) and shift (i.e. stress distribution) after annealing. This indicates that the stress within the guiding region is not relieved<sup>12</sup>. Crucially for the NV-waveguide device targeted in this work, we found that the mode profile and insertion loss of the annealed waveguides were unaltered, suggesting the temperature required to cause waveguide degradation is higher than that required to form the NVs.

Both the laser written optical waveguides and the laser written NVs are permanent and do not appear to degrade with photo bleaching or any other observed mechanism over time. The waveguides in particular have already demonstrated their robustness through surviving annealing up to temperatures of 1000  $^{\circ}\text{C}$ . All measured NV centers have remained photo

stable over several months of measurements including heated acid cleaning treatments and low temperature (4 K) spectroscopy.

## II. NV CENTER CHARACTERIZATION

Initial overhead photoluminescence (PL) characterization of the laser-written NV centers and their interaction with the waveguide was performed using a homebuilt confocal microscope. A fiber coupled 532 nm laser (CL532-500-L, CrystaLaser) was focused onto the sample through a 0.8 NA objective (100 $\times$  CFI60 TU Plan Epi ELWD, Nikon) mounted on a closed loop piezo stage (Triton 101, PiezosystemJena). The induced PL was collected through the same objective, filtered from the excitation and Raman scattered light using a dichroic beam splitter (ZT 532 RDC, Chroma) and long-pass filters (555 nm long-pass, ET 555 LP Chroma, 650 nm long-pass, FELH 0650 Thorlabs) to allow only the NV phonon sideband (PSB) to pass. This light was focused into a single mode fiber, providing the confocal aperture. Detection of the filtered light was performed using single photon avalanche photodiodes (SPQR-14, Perkin-Elmer). Fluorescence could also be directed to a spectrometer (Acton SP-2750, Princeton Instruments), or to a back-illuminated EMCCD (DU-897U-CS0-#BV iXon Ultra, Andor).

## III. NV CENTER CREATION STATISTICS

In order to find the required pulse energy for efficient NV formation, and to calibrate the writing depth relative to the waveguide formation depth, multiple test waveguides with trial static exposures were written. The number of NVs found at each at each trial point was characterized based on the confocal scan (whether there was a single bright spot), the depth of the  $g^{(2)}(0)$  dip in the intensity autocorrelation measurement, and the detected photon intensity at saturation.

The results from a total of 78 characterized trials are summarized in Figure 1, with 70 % confidence intervals calculated based on the number of trials tested in each case. The single NV center formation probability increases with pulse energy, however as the energy increases more, the probability of formation of multiple NV centers at the same site also increases. At 30 nJ multiple NV center formation appears to dominate. It should be noted however that

the formation probability is also dependent on the local density of nitrogen which can vary between samples and even between different sections of the same sample. These results are consistent with those in previous work<sup>13</sup>.

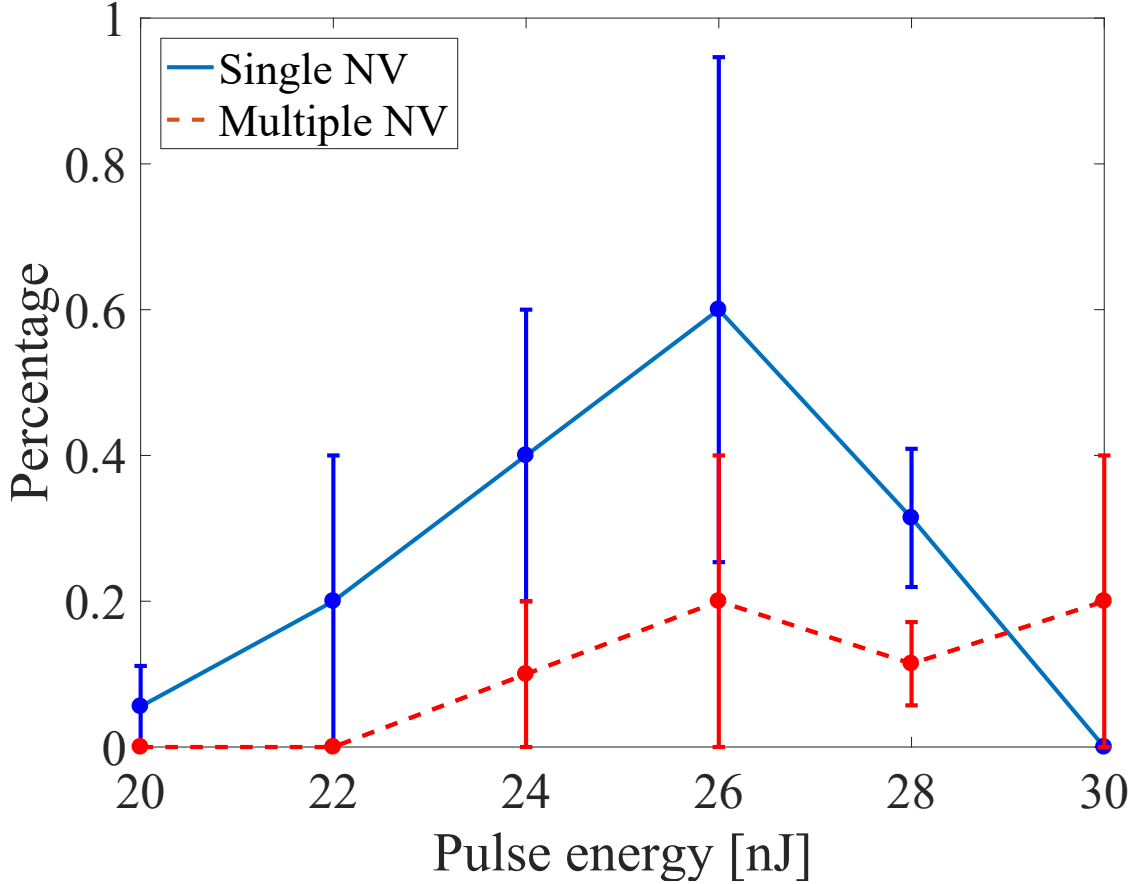

FIG. 1. NV center formation statistics showing the measured formation probability for single NV and multiple NV centers for increasing pulse energy.

#### IV. LOW TEMPERATURE NV CENTER SPECTRA

The low temperature line widths of NV centers are an important figure of merit for quantum applications, especially for applications which require indistinguishable coherent photons. Photoluminescence (PL) and Photoluminescence Excitation (PLE) spectra were recorded from the laser formed NV centers with the sample held at temperature  $\sim 6$  K inside a closed-cycle cryostat (Montana Nanoscale Workstation). A 0.5 NA long working distance objective was used with the previously described confocal microscope to image through the

cryostat window (60× G Plan Apo, Mitutoyo). Figure 2(a) and (b) show PL spectra from the NV2 demonstrating two spectrometer limited lines corresponding to the  $E_x$  and  $E_y$  orbital branches of the NV center's ZPL transitions<sup>14</sup>. The orbital lines show a splitting of 0.7 nm or 500 GHz, which is consistent with the effect of a stress field caused by the laser written modifications lines which define the waveguide<sup>2,15</sup>.

It is possible to use the stress induced splitting and shifting of the ZPL of stress as a probe of the local stress within the waveguide<sup>12</sup>. Grazioso et al. demonstrated the measurement of the full stress tensor within a bulk diamond sample using several neighboring NV centers experiencing the same stress field<sup>16</sup>. The splitting of an NV center under the stress tensor  $\sigma$  defined with (X,Y,Z) aligned with respect to the diamond's ([110], [-110], [001]) crystal axes is given by  $\delta = \sqrt{\beta^2 + \gamma^2}$  with  $\beta = B(2\sigma_{ZZ} - \sigma_{XX} - \sigma_{YY}) + C(\sigma_{YY} - \sigma_{XX} - \sqrt{2}\sigma_{YZ})$  and  $\gamma = 2\sqrt{3}B(\sigma_{XY}) - \sqrt{3/2}C(3\sigma_{XZ} - \sigma_{YZ})$ . The parameters B and C have been determined as  $-1.04 \text{ meV/GPa}$  and  $-1.69 \text{ meV/GPa}$ <sup>17</sup>.

With a single NV center it is not possible to achieve the full stress tensor measurement, however if we make the assumption that the dominant stress at the point of the NV center caused between the modification lines is compressive in the 100 direction ( $\sigma_{XX} \gg \sigma_{YY}, \sigma_{ZZ}, \sigma_{XY}, \sigma_{YZ}, \sigma_{ZX}$ ), we can estimate its magnitude to be of the order of 400 MPa, which is consistent with previous  $\mu$ Raman studies of similar waveguides<sup>2</sup>.

Figure 2(c) shows a photoluminescence excitation spectrum of one of the lines. In this measurement a tunable diode laser (New Focus) is used to scan across the ZPL transition at  $\sim 637 \text{ nm}$ , while monitoring the NV center's emission in the phonon side band (PSB). In order to improve the signal to noise ratio, multiple scans are averaged together, while a 532 nm laser is used to repump between scans. The PLE spectrum of NV2 shows two lines with widths of 500 MHz and 1800 MHz. The appearance of two or more lines is characteristic of an NV center undergoing spectral diffusion between scans, as local defects are ionized and change the local electric field experienced by the NV center. The cause of these defects is likely to be residual damage from the static writing pulse which has not been fully repaired by the annealing process. A line width of 500 MHz is an order of magnitude away from the NV center's 12 MHz Fourier transform limited line width, however it is consistent with the larger line widths Chen et al. measured at the upper end of their energy range<sup>13</sup>. Indeed it was reported that 50 % of the NV centers formed were so broad that PLE was not possible. Therefore it should be possible to achieve the lowest NV center line widths by reducing the

static exposure writing energy further.

Despite being written with three orders of magnitude greater fluence as compared to static exposures, NV centers were also formed in the vicinity of the laser modification lines making up the optical waveguide. This effect is due to the lower intensity in the wings of the focused Gaussian laser, and was also observed using picosecond laser irradiation of diamond<sup>18</sup>. These NV centers exhibit ZPLs with more splitting and which are much broader and less pronounced than the NV centers at the center of the waveguide. This suggests these NV centers are subject to higher strain and the effects of other local defects such as the GR1 center produced in the vicinity of the modification lines. An example spectrum of an NV center in the wings of the laser modification line is shown in Fig. 2 (d).

## V. ESTIMATED WAVEGUIDE NV COUPLING EFFICIENCY

We can make an estimate of the coupling between the NV center and the waveguide by considering  $\alpha = \frac{\Gamma_{wg}}{\Gamma_{tot}}$  the ratio of the spontaneous emission rate of a dipole into the waveguide  $\Gamma_{wg}$ , with the emission rate of a dipole in an isotropic medium  $\Gamma_{iso}$ .

The coupling efficiency between waveguides and single quantum emitters has been studied before, for example in the context of quantum dots coupled to photonic crystal or slot waveguides<sup>19,20</sup> and fluorescent dye molecules coupled to strip waveguides<sup>21</sup>. Here we review the derivation of the coupling efficiency, following the method of Quan et al<sup>20</sup>. The emission rate of a dipole  $\boldsymbol{\mu}$  positioned at  $\mathbf{r}$  at angular frequency  $\omega$  is given by Fermi's golden rule,

$$\Gamma = \frac{2\pi}{\hbar^2} |g(\omega, \mathbf{r})|^2 D(\omega) \quad (1)$$

where  $\hbar$  is the reduced Planck constant,  $g(\omega, \mathbf{r})$  is the dipole photon coupling strength and  $D(\omega)$  is the photonic density of states.

For a dipole in an isotropic medium with refractive index  $n = \sqrt{\varepsilon_r}$ , the coupling strength can be written  $g(\omega) = \sqrt{\frac{\hbar\omega}{2\varepsilon_r\varepsilon_0}} |\boldsymbol{\mu}| |\langle \hat{\boldsymbol{\epsilon}} \cdot \hat{\boldsymbol{\mu}} \rangle|$ , with  $\varepsilon_r$  the relative permittivity and  $\varepsilon_0$  vacuum permittivity, and we neglect the position  $\mathbf{r}$  of the dipole since it is in an isotropic medium. The scalar product of the unit vectors of the electric field and the dipole vector  $|\langle \hat{\boldsymbol{\epsilon}} \cdot \hat{\boldsymbol{\mu}} \rangle|^2 = \frac{1}{3}$  gives the dependence of the angle between the dipole and the electric field, averaged over all possible electric field orientations with respect to the dipole direction. The density of states

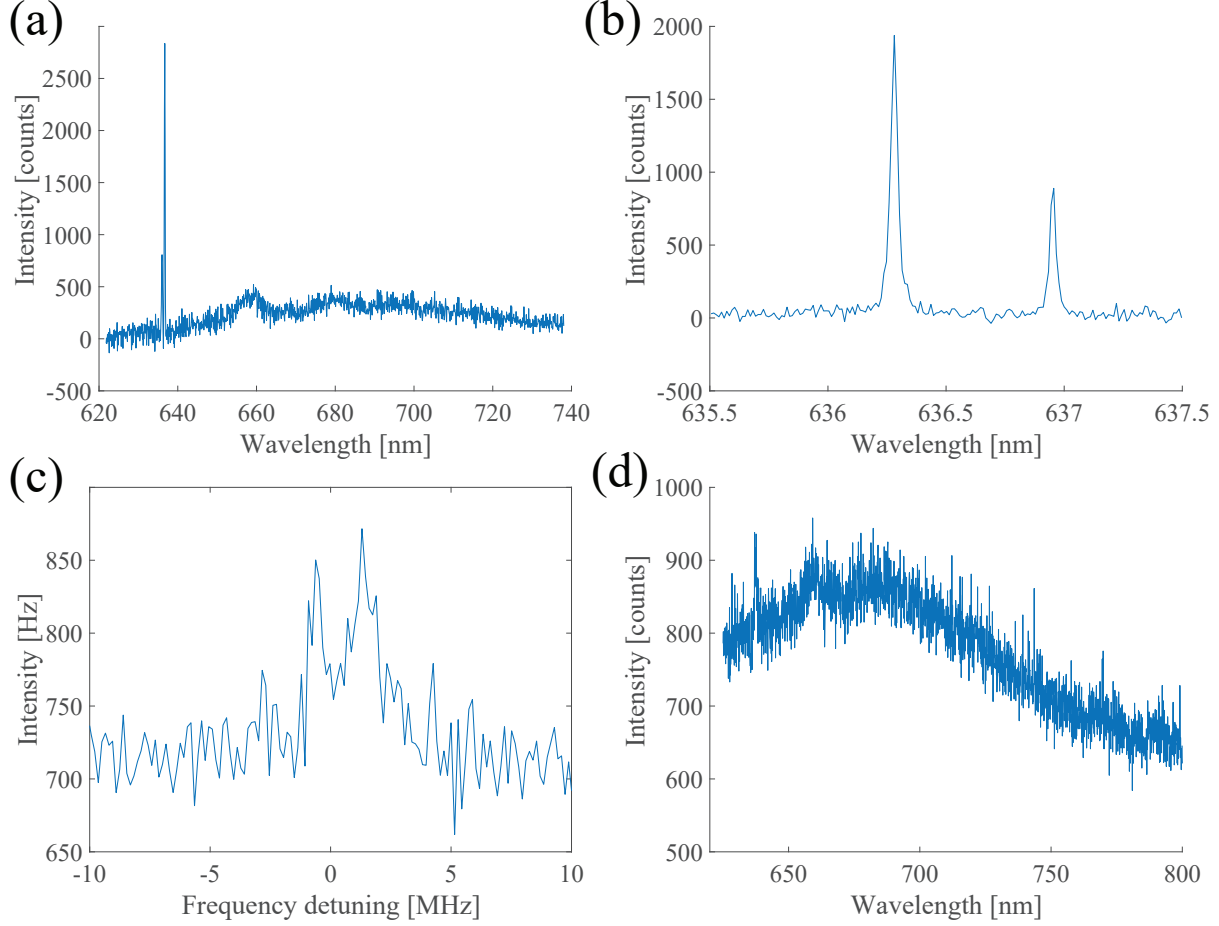

FIG. 2. NV center low temperature spectra. (a) Photoluminescence spectra of NV2 at  $\sim 6$  K. (b) High resolution photoluminescence spectra of NV2 showing split Ex and Ey orbitals. (c) Photoluminescence excitation spectrum of NV2. (d) Example spectrum of NV center at the edge of the waveguide.

is  $D(\omega) = \frac{\omega^2 n^3}{\pi^2 c^3}$ . Thus the total emission rate is

$$\Gamma_{iso} = \frac{n\omega^3}{3\pi\hbar\epsilon_0 c^3} |\boldsymbol{\mu}|^2. \quad (2)$$

We neglect local dielectric field corrections here<sup>23,24</sup> since they affect both  $\Gamma_{iso}$  and  $\Gamma_{wg}$  in the same proportion and so will not affect the ratio  $\alpha$ .

For the case of a dipole positioned within a waveguide, the coupling strength to a transverse waveguide mode is dependent on position and the orientation of the dipole with respect to the electric field of the guided mode, and can be written  $g(\omega, \mathbf{r}) = \sqrt{\frac{\hbar\omega}{2\epsilon_r\epsilon_0 A_{eff}(\mathbf{r}, \hat{\boldsymbol{\mu}})}} |\boldsymbol{\mu}| |\hat{\boldsymbol{\epsilon}} \cdot \hat{\boldsymbol{\mu}}|$ . Here the effective mode area,  $A_{eff}(\mathbf{r}_0, \hat{\boldsymbol{\mu}}) = \frac{\iint \epsilon_r(x, y) |\mathbf{E}(x, y) \cdot \hat{\boldsymbol{\mu}}|^2 dx dy}{\epsilon_r(\mathbf{r}_0) |\mathbf{E}(\mathbf{r}_0) \cdot \hat{\boldsymbol{\mu}}|^2}$

which can be interpreted as the confinement of the waveguide mode, so  $1/A_{eff}(\mathbf{r}_0, \hat{\boldsymbol{\mu}})$  is the normalized intensity at the point of the dipole. The density of states can then be obtained by noting the number of longitudinal modes in a one dimensional waveguide length  $L$  is  $\frac{L}{2\pi\nu_{gr}}$ , where  $\nu_{gr}$  is the group velocity, so  $D(\omega) = \frac{1}{2\pi\nu_{gr}}$ . Substituting into Fermi's golden rule again, we obtain the emission rate into one direction of the waveguide,

$$\Gamma_{wg} = \frac{\omega}{2\hbar\varepsilon_r\varepsilon_0\nu_{gr}A_{eff}(\mathbf{r}_0, \hat{\boldsymbol{\mu}})} |\hat{\mathbf{e}} \cdot \hat{\boldsymbol{\mu}}|^2 |\boldsymbol{\mu}|^2. \quad (3)$$

Finally we find the ratio of emission into a single direction of the waveguide to the total emission in an isotropic medium to be

$$\alpha = \frac{\Gamma_{wg}}{\Gamma_{iso}} = \frac{3\pi c^3}{2n^3\nu_{gr}A_{eff}(\mathbf{r}_0, \hat{\boldsymbol{\mu}})} |\hat{\mathbf{e}} \cdot \hat{\boldsymbol{\mu}}|^2 \quad (4)$$

$$\approx \frac{1}{4} \frac{\sigma_A}{A_{eff}(\mathbf{r}_0, \hat{\boldsymbol{\mu}})} (\cos(\theta))^2. \quad (5)$$

Here we make the approximation  $\nu_{gr} \approx c/n$  since most of the field is inside the waveguide mode, and the waveguide is only weakly guiding. The factor  $\sigma_A = \frac{3\lambda^2}{2\pi}$  is the scattering cross section for a dipole while  $\theta$  corresponds to the angle between the waveguide mode's electric field and the dipole transition matrix element. This equation indicates that the ratio of emission into the waveguide compared to the total emission of a dipole in an isotropic medium is proportional to the ratio of the scattering cross section and the waveguide's effective mode area.

If we approximate the waveguide mode's field with a Gaussian with FWHM = 5.9  $\mu\text{m}$  (corresponding to the  $\sim 10 \mu\text{m}$  MFD of the waveguide in this work measured at the  $1/e^2$  intensity point), the effective mode area is calculated as  $A_{eff}(\mathbf{r}_0, \hat{\boldsymbol{\mu}}) = 4.4 \times 10^{-11} \text{ m}^2$ . Therefore we obtain a ratio  $\alpha = 9 \times 10^{-4}$  with the parameters  $\lambda = 700 \text{ nm}$  (the center of the NV center phonon sideband),  $n = 2.42$  and  $\theta = 35.3^\circ$  (the angle between the waveguide's TM mode polarization and dipole plane perpendicular to the NV center's [111] symmetry axis), for an NV center  $|\mathbf{r}_0| = 1.2 \mu\text{m}$  from the center of the waveguide mode. Here we only consider the coupling of the NV center to the TM mode, since they do not support the TE mode<sup>2</sup>. Note that  $\alpha$  does not generally equal the true coupling efficiency because  $\Gamma_{tot}$  does not take into account the presence of the waveguide. For strongly guiding waveguides with smaller effective mode area, it is necessary to simulate the effect of the waveguide on  $\Gamma_{tot}$  using numerical

methods<sup>21</sup>, however for weakly guiding waveguides such as the laser written waveguides in this work, the effect will not be significant.

We can compare this coupling efficiency with the estimated collection efficiency of our confocal microscope objective. The collection efficiency of a microscope objective when collecting from an emitter hosted in a medium of refractive index  $n$  is  $\frac{1}{2}(1 - \cos(\phi))$ , where  $\phi = \sin^{-1}(\text{NA}/n)$  is the half angle of the collection cone. For the 0.8 NA microscope objective used in this work, we expect a collection efficiency of  $\sim 3\%$ . This suggests a waveguide collection efficiency  $\sim 0.03\%$  less than for the microscope objective.

The development of smaller MFD waveguides would increase the collection efficiency, assuming the waveguide loss does not substantially increase. For example a waveguide with a FWHM of  $1.1\text{ }\mu\text{m}$  (corresponding to a  $1/e^2$  MFD of  $1.9\text{ }\mu\text{m}$ ) would provide a collection efficiency of  $\sim 3\%$ , the same as for our microscope objective. It also may be possible to increase the collection efficiency by engineering the waveguide to reduce the group velocity  $v_{gr}$ , for example by the fabrication of Bragg grating waveguides<sup>19,25</sup>.

## VI. COMPARISON WITH EXPERIMENTAL DATA

Here we compare the theoretical predictions of the waveguide excitation relative power density reduction and the relative waveguide collection efficiency with experimental estimates taken from the results presented. Although these quantitative estimates are extracted from experimental data, they should be considered with some caution, since they rely on several assumptions including the theoretical performance of the microscope objective. They are also sensitive to the background correction and integration of the relatively signal, as well as long term drifts over the course of the experiment.

In the main paper it is noted that relative size of the waveguide mode compared to the size of the laser focused through a 0.8 NA objective into diamond ( $\text{FWHM}_{WG} = 5.9\text{ }\mu\text{m}$  and  $\text{FWHM}_M = \frac{2n\lambda}{\pi\text{NA}\sqrt{2\ln 2}} = 0.6\text{ }\mu\text{m}$  respectively) suggests that the effective power density of at the position of an NV center at the center of the beam will be a factor of 0.01 lower for the waveguide if the same power is used. We can compare this prediction with experimental data by estimating the excitation power in the waveguide at the position of the NV center under waveguide excitation and the power required to excite the same emission rate through confocal excitation.

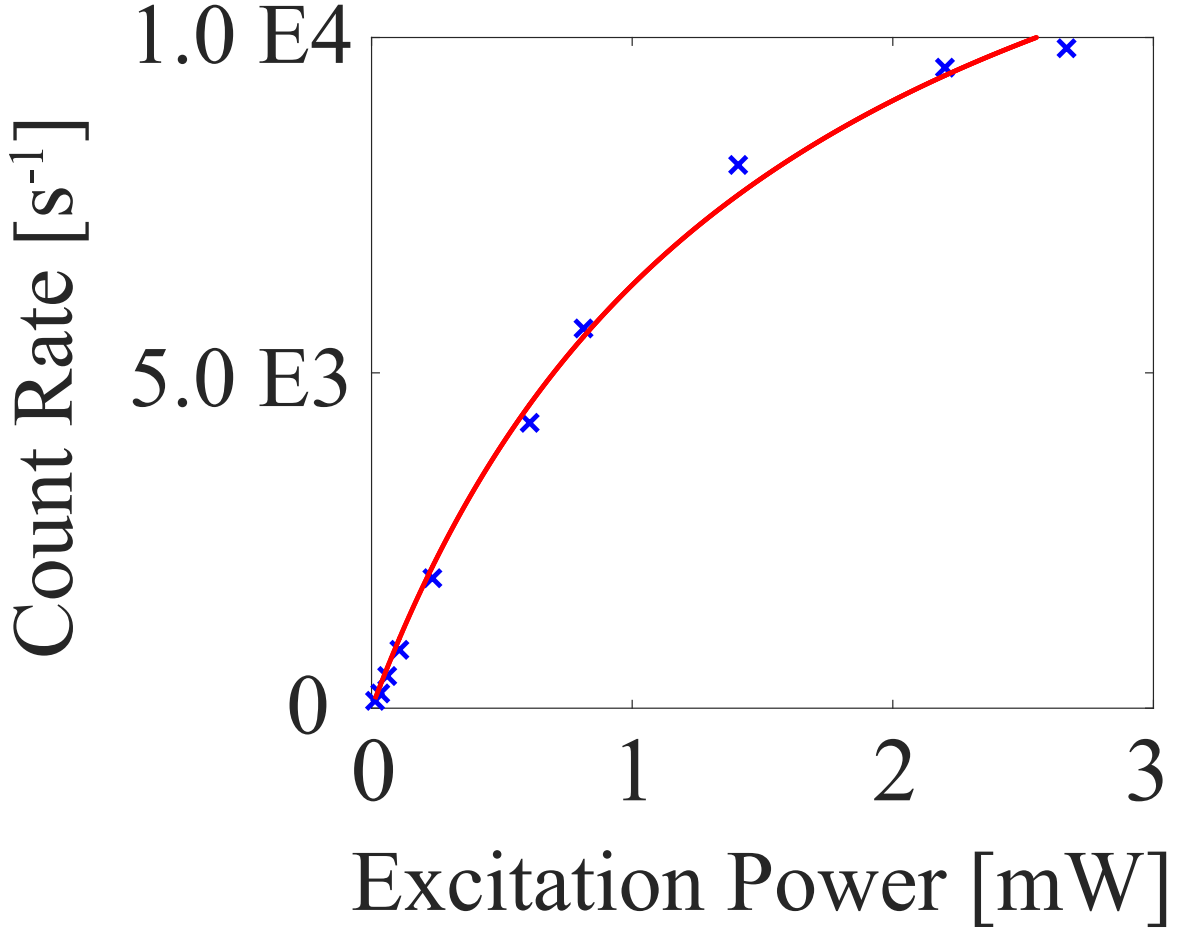

FIG. 3. Detected count rate from NV2 through confocal microscope as a function of excitation power. Measured data marked in blue, overlaid with a saturation fit in red.

In Figure 3(b) in the main paper, we observe that  $\sim 10$  photons per second are detected from the NV center through the confocal microscope when it is excited through the waveguide. During this measurement the transmitted 532 nm excitation light was monitored at the output facet of the waveguide, and was measured to be 165  $\mu\text{W}$ . We can infer 210  $\mu\text{W}$  laser excitation light in the waveguide at the position of the NV center based on the 4.2 dB/cm propagation loss rate, and the 1.6 dB loss due to Fresnel reflections at the diamond/air interface.

We estimate the relative excitation power through the confocal microscope objective by recording the detected photon count rate from NV2, corrected for background as a function of excitation power, and extrapolating to the low excitation power required for a  $\sim 10$  photons per second emission rate. This is shown in Fig. 3. The recorded data is

fitted to  $C = C_{Sat}P/(1 + P_{Sat})$ , where  $C$  is the detected count rate and  $P$  is the excitation power. The fit parameters  $C_{Sat}$  and  $P_{Sat}$  are the saturated count rate and saturation power (the power required to achieve  $\frac{1}{2}C_{Sat}$  counts) respectively. Through extrapolation, we can estimate the excitation power to achieve  $\sim 10$  photons per second as  $1\text{ }\mu\text{W}$ .

This suggests that the estimated reduction in effective power density for laser light in the waveguide as compared to that focused through microscope objective is 0.005. This is less than the value estimated from expected the relative sizes of the beams, however it is the correct order of magnitude. The discrepancy could be explained by several factors, including a mismatch between the orientation of the laser beam polarization in the waveguide and the NV center, as well as a difference in the mode shape for the 532 nm excitation light and the 637 nm design wavelength. It could also be due to the uncertainty associated with extrapolating the fitted count rate at low excitation powers.

We can also make a comparison between the theoretical relative waveguide collection efficiency and the experimental data by considering the integrated pixel count rates in Fig 3. (c) (when excited through the waveguide and collected through the confocal microscope objective) and Fig 3. (d) (when excited through the microscope objective and collected through the waveguide output facet). However, we cannot directly compare the two, since the excitation power density used in each case was different. Therefore we use the detected photon count rate through the confocal microscope using the single photon avalanche photodiodes (SPADs) in Fig. 3 (b) to calibrate the EMCCD's detection efficiency for the selected detection settings. We then are able to use the ratio of count rates we would expect to detect using SPADs in each case. In both cases the camera was operated at  $-80^\circ\text{C}$ , with a conventional gain of 3. The exposures were combined from several frames to allow for cosmic ray removal, and corrected by subtracting a background exposure.

For overhead collection from the NV center in Fig 3 (c) the total integrated pixel count was  $8.7 \times 10^3$  for a 600 s exposure (summing the pixels in  $1.5\text{ }\mu\text{m} \times 1.5\text{ }\mu\text{m}$  area around the NV center). This indicates a pixel count rate of  $\sim 14$  counts per second, and a detection rate of 1.4 EMCCD pixel counts per photon detected using the SPADs.

For waveguide collection from the NV center in Fig 3 (c) the total integrated pixel count was  $2.1 \times 10^6$  for a 4 h exposure (summing the pixels in  $9\text{ }\mu\text{m} \times 13\text{ }\mu\text{m}$  area around the waveguide output peak. This corresponds to a pixel count rate of  $\sim 150$  counts per second detected at the output facet using the EMCCD. This suggests that we would expect a count

rate of 110 counts per second using the SPADs if we collected through the waveguide. If we wish to compare this value to the theoretical relative collection efficiency, we must further correct for the 4.2 dB/cm propagation loss rate, giving an expected SPAD count rate of 120 counts per second collected into the waveguide excluding waveguide loss.

With the same 2.5 mW excitation power through the confocal microscope (overhead excitation, overhead collection), we detect  $\sim 10 \times 10^3$  photons per second using the SPADs. Thus the experimental relative collection efficiency is  $\sim 0.012$ . Again this value is less than the theoretically predicted value of 0.03. In this case the discrepancy could be attributed to the uncertainties associated with background correction and integration of the EMCCD exposures, since any small error is magnified by the number of pixels integrated over. In addition it could be due to simplifications in the theory, which modeled the NV center as a simple dipole.

## REFERENCES

- <sup>1</sup>J. Burghoff, C. Grebing, S. Nolte, and A. Tünnermann, *Appl. Phys. Lett.* **89**, 081108 (2006).
- <sup>2</sup>B. Sotillo, V. Bharadwaj, J. P. Hadden, M. Sakakura, A. Chiappini, T. T. Fernandez, S. Longhi, O. Jedrkiewicz, Y. Shimotsuma, L. Criante, R. Osellame, G. Galzerano, M. Ferrari, K. Miura, R. Ramponi, P. E. Barclay, and S. M. Eaton, *Sci. Rep.* **6**, 35566 (2016).
- <sup>3</sup>J. R. Rabeau, P. Reichart, G. Tamanyan, D. N. Jamieson, S. Praver, F. Jelezko, T. Gaebel, I. Popa, M. Domhan, and J. Wrachtrup, *Appl. Phys. Lett.* **88**, 023113 (2006).
- <sup>4</sup>B. Naydenov, F. Reinhard, A. Lämmle, V. Richter, R. Kalish, U. F. S. D’Haenens-Johansson, M. Newton, F. Jelezko, and J. Wrachtrup, *Appl. Phys. Lett.* **97**, 242511 (2010).
- <sup>5</sup>T. Yamamoto, T. Umeda, K. Watanabe, S. Onoda, M. L. Markham, D. J. Twitchen, B. Naydenov, L. P. McGuinness, T. Teraji, S. Koizumi, F. Dolde, H. Fedder, J. Honert, J. Wrachtrup, T. Ohshima, F. Jelezko, and J. Isoya, *Phys. Rev. B* **88**, 075206 (2013).
- <sup>6</sup>B. Sotillo, V. Bharadwaj, J. Hadden, S. Rampini, A. Chiappini, T. Fernandez, C. Armellini, A. Serpengüzel, M. Ferrari, P. Barclay, R. Ramponi, and S. Eaton, *Micromachines* **8**, 60 (2017).
- <sup>7</sup>Y.-f. Meng, C.-S. Yan, J. Lai, S. Krasnicki, H. Shu, T. Yu, Q. Liang, H.-k. Mao, and R. J.

- Hemley, Proc. Natl. Acad. Sci. **105**, 17620 (2008).
- <sup>8</sup>A. Benayas, D. Jaque, B. McMillen, and K. P. Chen, J. Appl. Phys. **107**, 033522 (2010).
- <sup>9</sup>A. Ródenas, G. A. Torchia, G. Lifante, E. Cantelar, J. Lamela, F. Jaque, L. Roso, and D. Jaque, Appl. Phys. B **95**, 85 (2009).
- <sup>10</sup>R. Kalish, A. Reznik, S. Praver, D. Saada, and J. Adler, Phys. status solidi **174**, 83 (1999).
- <sup>11</sup>A. C. Ferrari and J. Robertson, Phys. Rev. B **61**, 14095 (2000).
- <sup>12</sup>P. Olivero, F. Bosia, B. A. Fairchild, B. C. Gibson, A. D. Greentree, P. Spizzirri, and S. Praver, New J. Phys. **15**, 043027 (2013).
- <sup>13</sup>Y.-C. Chen, P. S. Salter, S. Knauer, L. Weng, A. C. Frangeskou, C. J. Stephen, S. N. Ishmael, P. R. Dolan, S. Johnson, B. L. Green, G. W. Morley, M. E. Newton, J. G. Rarity, M. J. Booth, and J. M. Smith, Nat. Photonics **11**, 77 (2016).
- <sup>14</sup>K.-M. C. Fu, C. Santori, P. E. Barclay, L. J. Rogers, N. B. Manson, and R. G. Beausoleil, Phys. Rev. Lett. **103**, 256404 (2009).
- <sup>15</sup>A. Batalov, V. Jacques, F. Kaiser, P. Siyushev, P. Neumann, L. J. Rogers, R. L. McMurtrie, N. B. Manson, F. Jelezko, and J. Wrachtrup, Phys. Rev. Lett. **102**, 195506 (2009).
- <sup>16</sup>F. Grazioso, B. R. Patton, P. Delaney, M. L. Markham, D. J. Twitchen, and J. M. Smith, Appl. Phys. Lett. **103**, 101905 (2013).
- <sup>17</sup>G. Davies and M. F. Hamer, Proc. R. Soc. A Math. Phys. Eng. Sci. **348**, 285 (1976).
- <sup>18</sup>S. M. Pimenov, A. a. Khomich, B. Neuenschwander, B. Jäggi, and V. Romano, J. Opt. Soc. Am. B **33**, B49 (2016).
- <sup>19</sup>V. S. C. Manga Rao and S. Hughes, Phys. Rev. B **75**, 205437 (2007).
- <sup>20</sup>Q. Quan, I. Bulu, and M. Lončar, Phys. Rev. A **80**, 011810 (2009).
- <sup>21</sup>J. Hwang and E. A. Hinds, New J. Phys. **13**, 085009 (2011).
- <sup>22</sup>M. Fox, *Quantum Optics, An Introduction*, Vol. 67 (Oxford University Press, 2006) p. 441.
- <sup>23</sup>S. M. Barnett, B. Huttner, and R. Loudon, Phys. Rev. Lett. **68**, 3698 (1992).
- <sup>24</sup>K. Dolgaleva and R. W. Boyd, Adv. Opt. Photonics **4**, 1 (2012).
- <sup>25</sup>V. Bharadwaj, A. Courvoisier, T. T. Fernandez, R. Ramponi, G. Galzerano, J. Nunn, M. J. Booth, R. Osellame, S. M. Eaton, and P. S. Salter, Opt. Lett. **42**, 3451 (2017).
